# Supplementary material for: DreamTalk: When Emotional Talking Head Generation Meets Diffusion Probabilistic Models
Source: arXiv:2312.09767 source file (2024-08-10)
Supplement: Supplementary file 1 [file 02_additional_results_for_expressive_talking_head_generation.tex]

\section{Additional Results for Emotional Talking Head Generation}

\subsection{Analysis on Generalization Capabilities}
\label{sec:analysis_on_generalization_capabilities}

\noindent\textbf{Songs.}
As demonstrated in \suppvideo, our method successfully generates reasonable results for songs, even those with accompaniment, despite this being significantly different from the training dataset's data distribution. A noticeable decline in lip-sync accuracy is observed when the accompaniment volume is excessively high. We conduct a comparative analysis of lip-sync performance between songs with accompaniment and songs with removed accompaniment (using data from the SingFace Dataset~\cite{liu2023musicface}). It is found that the accompaniment adversely affects lip-sync, leading to mouth movements resembling mumbling. Addressing the negative impact of accompaniment on lip-sync accuracy presents an interesting avenue for future research.
% As shown in \suppvideo, our method is able to generate reasonable results for songs even with accompaniment, which is far from the data distribution of the training dataset. We observe a performance drop on lip-sync when the accompaniment is too loud. We compare the lip-sync performance of results generated using Songs with accompaniment and Songs with the accompaniment removed (from SingFace Dataset~\cite{liu2023musicface}) and observe that the accompaniment compromises the lip-sync, dragging the mouth to mumbling motions. How to reduce the adverse effect of accompaniment on lip-sync is leaved for future research.

\noindent\textbf{Speech in Multiple Languages.}
\suppvideo shows that our method generates satisfactory results with speech in French, Chinese, Spanish, German, Italian, Japanese, and Korean. The versatility of wav2vec features aids application across various languages. Additionally, the inclusion of multilingual talking head videos from Voxceleb2 enhances generalization.
% The supplementary video demonstrates that our method effectively generates results with French, Chinese, Spanish, Italian, Japanese, and Korean speech. Wav2vec's versatile features enable application across various languages. 

\noindent\textbf{Noisy Audio.}
% \suppvideo shows that our method generates satisfactory results with audio that is noised with different types of noise and different noise intensity levels.
% We use the noise recorded in a meeting, in the office and in the cafeteria, which are the common environment for talking head applications,  from DEMAND dataset~\cite{thiemann2013diverse} and mix the audio with noise using an off-the-shelf software \footnote{\url{https://github.com/Sato-Kunihiko/audio-SNR}} at SNR 20dB, 10dB, and 0dB. We observe no noticeable performance drop even at 0dB, where the noise is as loud as the speech and causes a significant decrease in the intelligibility and clarity of the speech.
\suppvideo demonstrates that our method yields satisfactory outcomes when processing audio mixed with multiple noise types and intensities. We employ noise recordings from typical talking head application environments—meetings, offices, and cafeterias—sourced from the DEMAND dataset~\cite{thiemann2013diverse}. We blend the audio with noise at several SNRs and test the performance. We found that our method maintains performance even at 0 dB SNR, where the noise is as loud as the speech and significantly impairs speech intelligibility and clarity.

\begin{figure}[t!]
  \centering
  \includegraphics[width=0.47\textwidth]{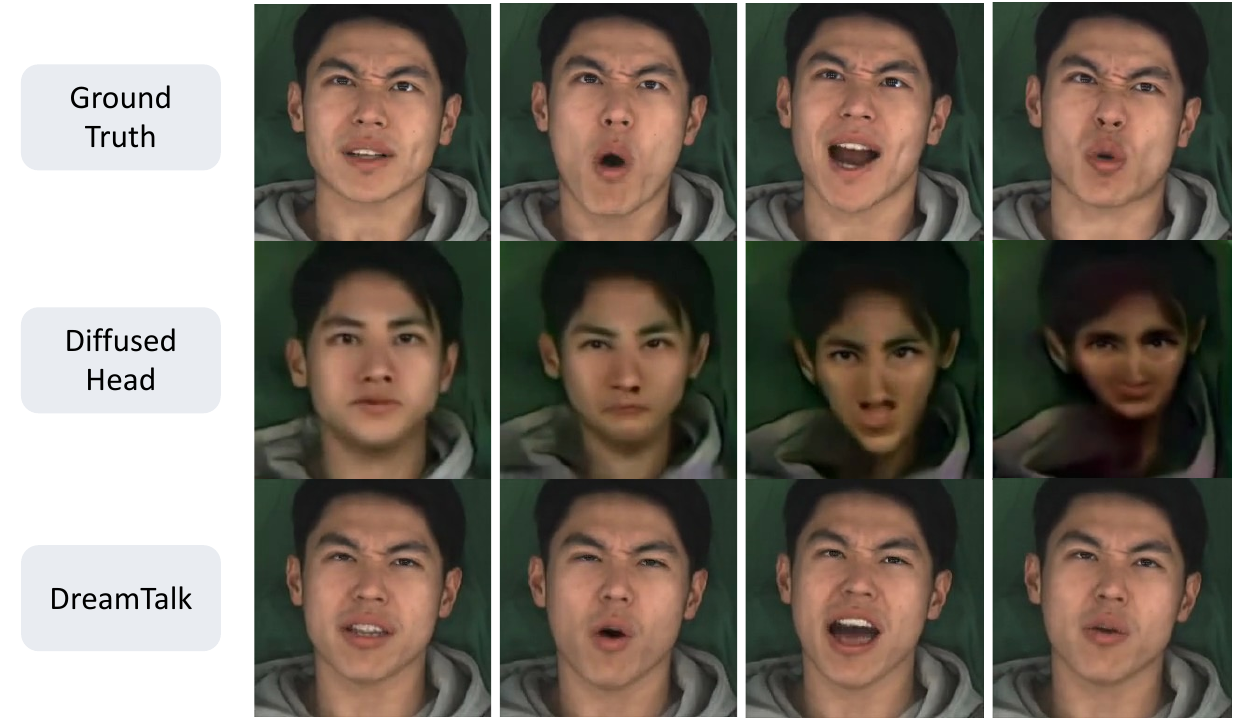}
  % \vspace{-3mm}
  \caption{Comparisons with Diffused Head. Diffused Head frequently generate distorted faces and warped images.}
  \label{fig:compare_with_diffused_head}
  % \vspace{-2mm}
  % \vspace{-0.1cm}
\end{figure}

\subsection{More Comparisons with Diffused Head and TH-PAD}
We compare our method with Diffused Head~\cite{stypulkowski2023diffused} and TH-PAD~\cite{yu2023talking}, two diffusion-based methods,  on MEAD. For a fair comparison, we use audio to specify the styles used by DreamTalk. \cref{table:compare_with_thpad_dh} shows that DreamTalk achieves the best scores. 
The expressions produced by TH-PAD only synchronize with the audio rhythm but do not match the audio's emotion. Although TH-PAD is also trained on datasets with emotional expressions, TH-PAD focuses on expression diversity but does not consider the alignment with the audio's emotional content, while achieving emotional alignment is a more difficult task. We also observe that TH-PAD often changes the speaker identity. Diffused Head can only generate discrete types of emotions and cannot control the personalized variations of emotions. It also frequently generates distorted faces and warped images, shown in \cref{fig:compare_with_diffused_head}, which may be due to the buildup of errors across the sequence of generated frames.

\begin{table}[t]
% \small
\centering
\caption{Comparisons with Diffused Head and TH-PAD. DreamTalk(A) uses styles inferred from audio.}
\setlength{\tabcolsep}{0.5mm}{
\begin{tabular}{cccccc}
% \toprule  
Method & SSIM$\uparrow$ & CPBD &F/M-LMD$\downarrow$ & SA$\uparrow$ & $\text{Sync}_{\text{conf}}$$\uparrow$ \\
% \midrule
\shline
Diffused Head   & 0.54 & 0.08 & 5.61/6.85 &  22.6  &  1.87 \\

TH-PAD & 0.46 & 0.05 & 6.38/5.81 & 5.3 & 2.42 \\

\textbf{DreamTalk(A)}  & \textbf{0.84} & \textbf{0.16} & \textbf{2.24}/\textbf{3.43} &  \textbf{78.6}  & \textbf{3.73}\\

\textcolor{gray}{GT} & \textcolor{gray}{1} &  \textcolor{gray}{0.22} & \textcolor{gray}{0}/\textcolor{gray}{0} & \textcolor{gray}{92.5} & \textcolor{gray}{4.13} \\ 

% \bottomrule 
\end{tabular}}

\label{table:compare_with_thpad_dh}
\end{table}

\subsection{More ablation studies}

\begin{table}[t]
% \small
\centering
\caption{The additional results of DreamTalk's ablation study on MEAD.}
\setlength{\tabcolsep}{0.5mm}{
\begin{tabular}{ccccc}
% \toprule  
Method & SSIM$\uparrow$ & F-LMD$\downarrow$ & M-LMD$\downarrow$  & $\text{Sync}_{\text{conf}}$$\uparrow$ \\
% \midrule
\shline
% w/o Lip Expert   & 0.85 & \textbf{1.90} & 3.07   &  2.63 \\
% Uncond Lip Expert  & 0.83 & 2.19 & 3.42    & \textbf{4.51}\\
w/o Diffusion  & 0.82 & 2.25 & 3.39    & 3.18 \\
Blend. Lip Expert  & 0.83 & 2.10 & 3.03    & 3.32 \\
% \cmidrule(r){1-5}
\textbf{Full} & \textbf{0.86}  &  \textbf{1.93} & \textbf{2.91}   & \textbf{3.78} \\

% \bottomrule 
\end{tabular}}

\label{table:more_ablation_study}
\end{table}

To further validate the effectiveness of our design, we conduct an ablation study with two variants: (1) replace the diffusion model with a GAN model that uses the same architecture but is trained using GAN loss and regression loss(\textbf{w/o Diffusion}); (2) use the 3DMM expression parameters (blendshapes) as the input of lip expert, instead of using only the vertices in the mouth area(\textbf{Blend. Lip Expert}).

\cref{table:more_ablation_study} shows the results. \textbf{w/o Diffusion} cannot consistently generate correct emotional expressions and accurate lip-sync for diverse speaking styles (\suppvideo shows an example), potentially due to GAN's mode-collapse issue. Its scores are all lower than \textbf{Full}. This validates diffusion models' superiority over GANs in emotional talking head generation. \textbf{Blend. Lip Expert} also has degraded performance in generating emotional expressions and lip-sync. This is because, within the blendshapes, information about the mouth shape is mixed with that of other facial features. Therefore, when training a lip expert with blendshapes as input, information from other parts of the face can interfere with the accurate judgment of mouth shapes. The result validates the necessity of using mouth vertices as the input for the lip expert.

\subsection{Style Code Interpolation.}
\label{sec:style_code_interpolation}
Leveraging the style space, we can modify speaking styles via style code manipulation. \cref{fig:interpolation} illustrates that linear interpolation between style codes results in a seamless transition of generated speaking styles. This interpolation process allows for style intensity modulation and the generation of novel speaking styles.

\begin{figure}[t!]
  \centering
  \includegraphics[width=0.47\textwidth]{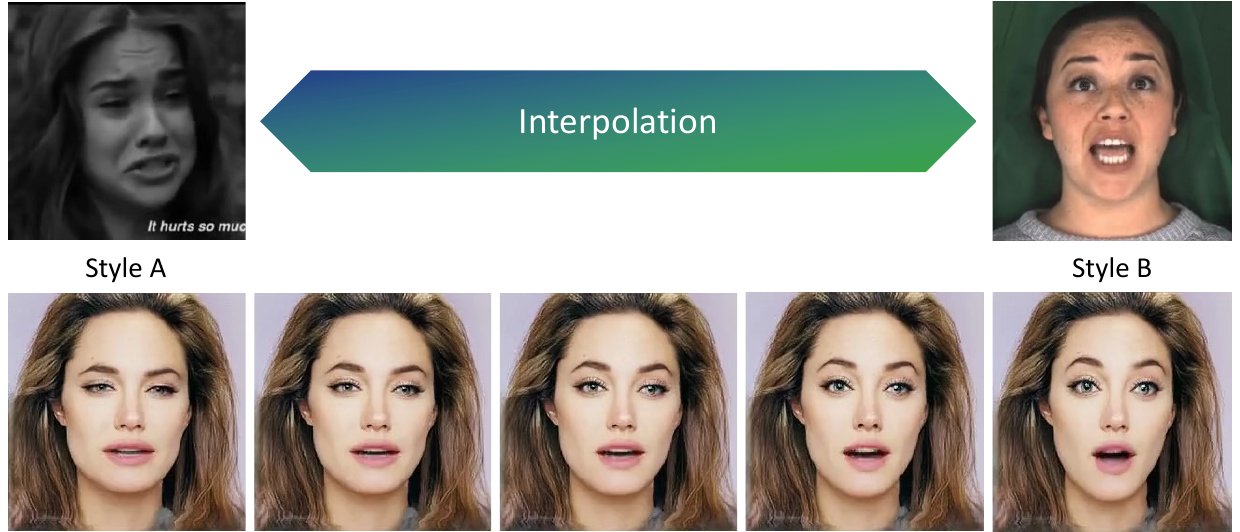}
  % \vspace{-3mm}
  \caption{The results of speaking style interpolation.}
  \label{fig:interpolation}
  % \vspace{-2mm}
  % \vspace{-0.1cm}
\end{figure}

\subsection{More Results of Style Code Visualization}
\label{sec:more_results_of_style_code_visualization}

\begin{figure}[t!]
  \centering
  \includegraphics[width=0.47\textwidth]{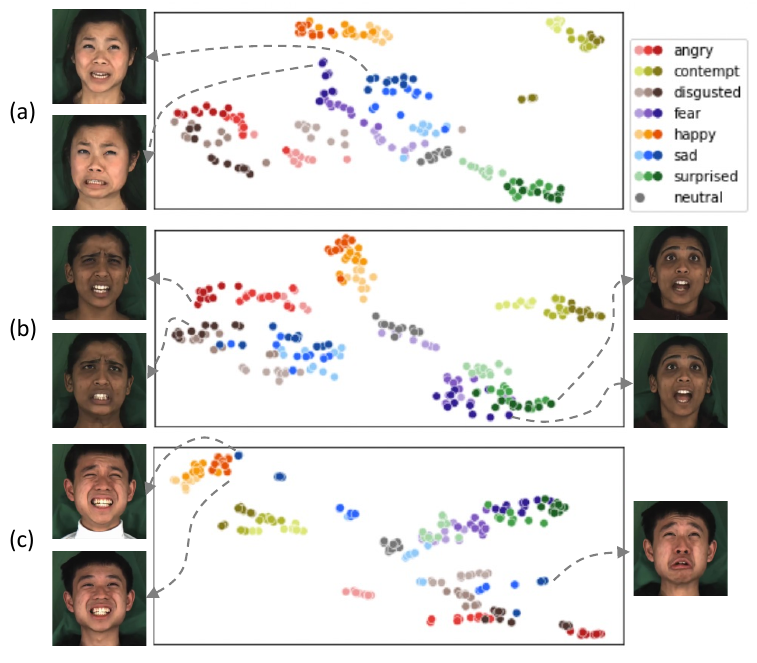}
  % \vspace{-4mm}
  \caption{t-SNE visualization of style codes for 3 speakers, with darker hues representing increased emotional intensity.}
  \label{fig:personalized_style_code_visualization}
  % \vspace{-0.1cm}
\end{figure}
We observe that each speaker's style code distribution exhibits both common patterns and individualized characteristics. Common patterns include: Firstly, speaking styles of different emotions cluster together first, with styles of lower intensity being closer to neutral and those of higher intensity being further away. Secondly, speaking styles of anger and disgust, as well as fear and surprise, often cluster together, as shown in \cref{fig:personalized_style_code_visualization}~(b) and (c).  Note that unlike \cite{ma2023styletalk}, our method does not incorporate losses to constrain style space.

\cref{fig:personalized_style_code_visualization}~(a) illustrates an example of individualized characteristics. The speaker's manifestation of fear closely resembles sadness, lacking the characteristic wide-eyed and open-mouthed expression, thereby positioning the speaking styles of fear nearer to those of sadness rather than surprise. Even within the same emotion, a speaker's speaking style can exhibit notable variation.
In \cref{fig:personalized_style_code_visualization}~(c), the speaker's dual expression of sadness—once with clenched teeth, similar to happy expressions, and another with depressed lip corners, akin to disgust—results in style codes close to the respective emotions. This observation diminishes the rationale for manually categorizing styles based on emotion and intensities in \cite{ma2023styletalk}.

\subsection{Generating emotions with personalized variations}

\begin{figure}[t!]
  \centering
  \includegraphics[width=0.47\textwidth]{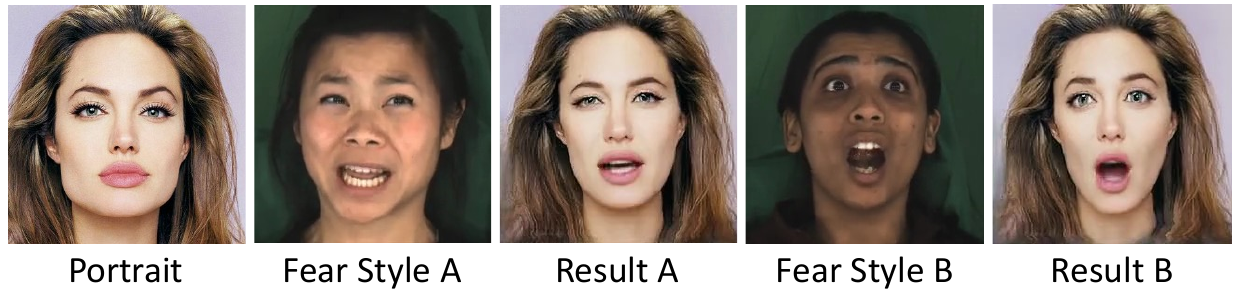}
  % \vspace{-4mm}
  \caption{DreamTalk can generate emotions with personalized variations.}
  \label{fig:personalized_emotions}
  % \vspace{-0.1cm}
\end{figure}

As shown in \cref{fig:personalized_emotions}, different persons express a single type of emotion with different expressions, and DreamTalk can generate emotions with such personalized variations. Fear style A conveys the emotion through narrowed eyes, whereas style B manifests it with eyes and mouth wide open. DreamTalk accurately generated the corresponding facial expressions.

% \subsection{Discussions Regarding Diffusion-based Methods}

% Recently, a few talking head generation methods~\cite{tian2024emo,stypulkowski2023diffused,shen2023difftalk,yu2023talking,du2023dae} have started to explore the use of diffusion models.
% Most methods utilize diffusion models to directly generate the image pixels, while DreamTalk adopts a different approach: it first uses diffusion models to generate audio-driven facial motions and then converts the motions into images. This design is based on our belief that learning the mappings from audio to motion and from motion to image separately is easier than directly learning the mapping from audio to image. An audio segment is more closely related to the facial motions, such as the opening and closing of the mouth, and less related to the specific colors of image pixels, such as black or white. Although such a two-stage design's performance may be limited by the expressiveness of the face representation~\cite{tian2024emo}, the ease of learning facilitates the model to learn accurate and vivid face motions. The advantage is more important for emotional talking head generation since it is a more severe one-to-many mapping problem and hence is more challenging to learn. The two-stage design eases the learning difficulty and hence allows DreamTalk to achieve high-quality results across diverse emotions.
