# Supplementary material for: DreamTalk: When Emotional Talking Head Generation Meets Diffusion Probabilistic Models
Source: arXiv:2312.09767 source file (2024-08-10)
Supplement: Supplementary file 2 [file 03_implementation_details.tex]

\section{Implementation Details}

\subsection{Architectual Details}

\subsubsection{Denoising Network} The audio encoder processes an input window of 11 sequential audio features, each of dimension $1024$. These features undergo dimension reduction to $256$ via a linear layer and then are fed to a transformer encoder comprising three 8-head transformer encoder layers, each with a hidden size of 256. Subsequently, a linear layer transforms the output tokens to yield audio tokens sized $11 \times 256$. The audio tokens are concatenated with noisy motion and then added with the encoded diffusion step.

The style encoder ingests sequential expression parameters from style reference videos, each sequence sized $N \times 64$. These sequences, ranging in length from 64 to 256 frames, are initially expanded to 256 dimensions via a linear layer. Subsequently, they are introduced into a transformer encoder, composed of three 8-head layers, each with a hidden size of 256. The resulting output tokens, each with a dimension of $256$, are aggregated through self-attention pooling~\cite{safari2020self}, yielding a style code of dimension $256$.

Within the decoder, the style code is repeated $11$ times, subsequently added with positional embedding to produce style tokens. These tokens, in conjunction with audio tokens, are processed by a transformer decoder, encompassing three 8-head layers, each with a hidden dimension of 256. Here, style tokens serve as the query, while audio tokens serve as both key and value. The middle output token is fed into a linear layer to predict facial motion.

% For implementation, inspired by ~\citet{ma2023styletalk}, we segregate expression parameters into lower and upper facial groups. Two parallel decoders are then employed to predict their respective groups. The resultant outputs are combined to derive the final facial motion.

\subsubsection{Style-aware Lip Expert}
\begin{figure}[t!]
  \centering
  \includegraphics[width=0.47\textwidth]{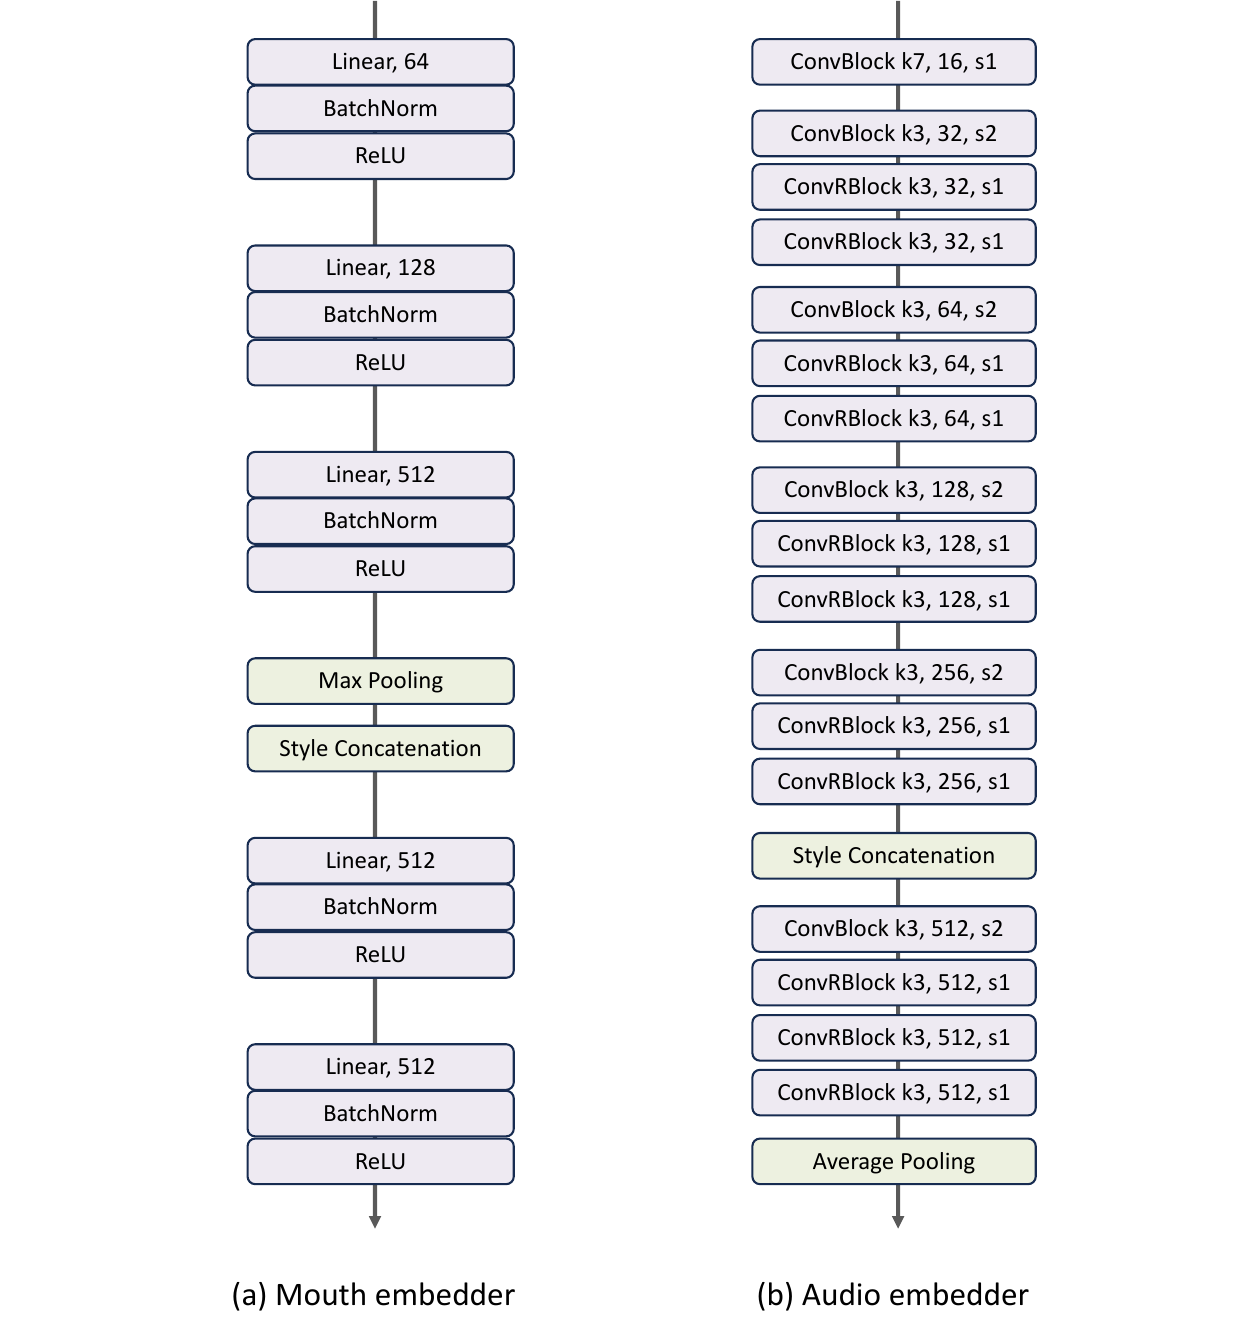}
  % \vspace{-3mm}
  \caption{The architecture of mouth embedder and audio embedder. ConvBlock consists of a 1D CNN layer, a batch normalization layer, and a ReLU layer. "k3, 32, s2" means that the kernel size is 3, the output dimension is 32, and the stride is 2. ConvRBlock is a ConvBlock with residual connection.}
  % \vspace{-2mm}
  \label{fig:lip_expert_architecture}
  % \vspace{-0.1cm}
\end{figure}
The face mesh is obtained by adding the mean shape to the product of the expression parameters and expression bases.
\cref{fig:lip_expert_architecture} shows the architecture of the audio embedder and the mouth embedder. Both embedders incorporate a ReLU layer as their final layer to ensure the output remains positive. This guarantees that the cosine similarity of the outputs falls within the valid probability range of $[0, 1]$.

\subsubsection{Style Predictor}
The style predictor is implemented as a transformer encoder comprising six 8-head transformer encoder layers, each with a hidden size of $256$. The input features are all linearly projected to $256$.

\subsection{Data Details}
\subsubsection{Datasets}

\noindent\textbf{MEAD.} The dataset, an in-lab talking-face corpus, features 60 speakers articulating eight emotions at three different intensity levels. When dividing the MEAD dataset into training and test subsets, we adhere to previously established methodologies~\cite{ji2022eamm}.

\noindent\textbf{HDTF.}
The dataset stands out as a high-resolution, in-the-wild audio-visual dataset. We designate $10\%$ of HDTF videos for testing and reserve the remainder for training.

\noindent\textbf{Voxceleb2.}
Voxceleb2 is a large-scale talking head dataset with videos collected from YouTube. We redownload and recrop the videos to improve their resolution to $256\times256$. Subsequently, approximately $80000$ high-quality videos are selected, with $400$ allocated for testing and the rest for training.

\noindent\textbf{RAVDESS.}
The dataset features 24 professional actors (12 female, 12 male) vocalizing two 
lexically matched statements in a neutral North American accent. It encompasses a range of expressions in both speech and song, each articulated at two levels of emotional intensity, with an additional neutral expression included. We employ the speech data from RAVDESS, encompassing eight emotions, for evaluation.
% For style predictor, The division of training and test sets on the MEAD dataset aligns with the procedure employed for \method. 

\subsubsection{Data Processing}
The original videos are cropped and resized to $256\times256$ pixels, aligning with the specifications in FOMM \cite{siarohin2019first}, and are sampled at 25 FPS. The 3DMM parameters are extracted by Deep3DFace~\cite{deng2019accurate}.

Regarding the audio features used in the denoising network and the style-aware lip expert, we downsample the speech wave into the sampling rate of 16000 and extract acoustic features employing a pre-trained Wav2Vec2.0 model~\cite{baevski2020wav2vec}.

For audio features used in the style predictor, we extract them using a pre-trained HuBERT model~\cite{hsu2021hubert}. Besides, we also utilize low-level audio features including Mel Frequency Cepstrum Coefficients (MFCC), Mel-filterbank energy features (FBANK), fundamental frequency, and voice flag. These two type of features are concatenated to represent the audio features used in the style predictor.

\subsection{Evaluation Details}

\subsubsection{Style Accuracy Metric}
\label{sec:style_accuracy_metric}
The style classifier used in Style Accuracy (SA) is applied to 3DMM face motions. We evaluate this metric on MEAD only since the number of RAVEDESS videos for each style is inadequate to train a style classifier. We put the videos from the same speaker, emotion, and intensity into one style and train a style classifier to classify which style a face motion sequence belongs to. The style classifier is constructed mainly using 1D-CNNs.  For methods that do not generate 3DMM, we extract 3DMM from their results for evaluation.

\subsection{Training Details}

Our framework is implemented on Pytorch. We employ Adam~\cite{kingma2014adam} for optimization, with a learning rate set to $0.0001$. The number of diffusion steps for the denoising network and style predictor is $1000$. The training batch size for the denoising network, style predictor, and lip expert is $64$, $64$, and $32$, respectively. $\lambda_{\text{denoise}}$, $\lambda_{\text{sync}}$, $n$, and $w$ are set to $1$, $1$, $5$, and $5$, respectively. The number of frames for style reference and audio used in style prediction is limited to $64 - 256$, corresponding to a time length of $2.56 - 10.24$ seconds. The denoising network, style predictor, and lip expert are trained on one NVIDIA Tesla A100 GPU for about $3$, $1$, and $10.5$ hours, respectively.

\subsubsection{Finetuning PIRender}
The renderer is fine-tuned with the losses in ~\cite{ren2021pirenderer} using MEAD. Instead of training with the self-reconstruction protocol where the source frame and target frame are from the same video, we select the source frame and target frame from the same speaker with different emotions. This enables the renderer to generate emotions different from the input portrait. This also allows our method to utilize portraits with emotions, unlike previous approaches that are confined to using neutral portraits~\cite{ji2022eamm}. We incorporate some neutral videos in Voxceleb into the data used for fine-tuning, which enhances the performance in identity preservation.

% \subsubsection{Training Style-aware Lip Expert}
% The style-aware lip expert is trained to discriminate whether the input audio and face motions are synchronized. We use cosine-similarity with binary cross-entropy loss to train the lip expert. Specifically, we compute cosine-similarity for the face motion embedding $\vect{e}^m$ and audio embedding $\vect{e}^a$ to represent the probability that the input audio-motion pair is synchronized. The training loss of the lip expert is: 
% \begin{equation}
%     \mathcal{L}_{\eqword{expert}} =\eqword{BCE}( \frac{\vect{e}^m\cdot \vect{e}^a}{\max (||\vect{e}^m||_2\cdot||\vect{e}^a||_2 , \epsilon )}),
% \end{equation}
% where $\epsilon$ is a small number for avoiding the division-by-zero error.

\subsection{Inference Details}
The inference of the denoising network can be accelerated with DDIM. We generate samples with $10$ DDIM steps and observe no performance drop. Generating a 30-second video offline takes $15.61$ seconds, with the face motion generation only taking $1.24$ seconds. During evaluation, the scale factor $\omega$ of classifier-free guidance is set to $1$. The style predictor uses the sampling algorithm of DDPM to predict style codes.

The emotion conveyed in the style reference (video or audio), should remain consistent to avoid confusing the model.

The head pose information, which is fed into the renderer, can be derived from real videos or generated using existing methods~\cite{wang2021audio2head}.
