# Supplementary material for: DreamTalk: When Emotional Talking Head Generation Meets Diffusion Probabilistic Models
Source: arXiv:2312.09767 source file (2024-08-10)
Supplement: Supplementary file 3 [file 06_ethical_consideration.tex]

\section{Ethical Consideration}

\method is able to generate realistic talking head videos. This positions \method with a broad spectrum of potential applications, each carrying intricate societal implications. While \method holds significant potential in amplifying and enriching human creative endeavors and may pave the way for innovative tools for creative professionals, its capabilities also harbor risks. There's a possibility for \method to generate content that might encompass or imply sexual themes, promote hatred, or depict violence. Misuse of \method could lead to negative repercussions on individuals or groups, potentially erasing or maligning them, perpetuating stereotypes, and subjecting them to disrespect. Other concerns include the potential for harassment, intimidation, or exploitation. Furthermore, \method's capabilities might be harnessed to mislead or spread misinformation.

Before releasing \method, we have implemented and plan to introduce several safeguards to curb potential misuse. Users will be advised against using images without the depicted individuals' consent to combat harassment and bullying. To prevent the spread of misinformation, all \method outputs will bear watermarks indicating their synthetic nature. Our commitment remains steadfast in continuously researching ways to minimize adverse societal effects.
