# Supplementary material for: DreamTalk: When Emotional Talking Head Generation Meets Diffusion Probabilistic Models
Source: arXiv:2312.09767 source file (2024-08-10)
Supplement: Supplementary file 5 [file 04_applications.tex]

\section{Applications}

Talking head for ChatGPT.
apply to other facial 3DMM and avatar
\todo{refer to GestureDiffuCLIP and MakeItTalk}
