# Supplementary material for: DreamTalk: When Emotional Talking Head Generation Meets Diffusion Probabilistic Models
Source: arXiv:2312.09767 source file (2024-08-10)
Supplement: Supplementary file 7 [file preamble.tex]

%
% --- inline annotations
%
\usepackage[dvipsnames]{xcolor}

\usepackage{colortbl} 
% \usepackage{xcolor}
\newcommand\wx[1]{{\color{blue}#1}}
\newcommand\zsw[1]{{\color{orange}#1}}
\newcommand{\red}[1]{{\color{red}#1}}
\newcommand{\todo}[1]{{\color{red}#1}}
\newcommand{\TODO}[1]{\textbf{\color{red}[TODO: #1]}}
% --- disable by uncommenting  
% \renewcommand{\TODO}[1]{}
% \renewcommand{\todo}[1]{#1}

\usepackage{cleveref}

\usepackage{graphicx}
\usepackage{tabularx}
\usepackage{makecell}
\usepackage{subcaption}
\usepackage{multirow}
%\usepackage{gensymb}
\usepackage{amsmath}
\usepackage{amssymb}
%\usepackage{amssymb}
%\usepackage{mathtools}
\usepackage{mathrsfs}
\usepackage{bm}

\usepackage[T1]{fontenc}
\usepackage{indentfirst} % added by wx


\newcommand{\isep}{\mathrel{{.}\,{.}}\nobreak}
\newcommand{\vect}[1]{\bm{#1}}

\usepackage{booktabs}
% \usepackage{natbib}
\usepackage{xspace}

\newcommand{\method}{DreamTalk\xspace}
% \newcommand{\stylespec}{style predictor\xspace}

\newcommand{\eqword}[1]{{\text{#1}}}
\newcommand{\norm}[1]{\lVert #1 \rVert}
\newcommand{\absvalue}[1]{\lvert #1 \rvert}


\newcommand{\fig}{Figure{}~}
\newcommand{\eqn}{Equation{}~}

\newcommand{\supp}{\textit{Supp. Mat.}\xspace}
\newcommand{\suppvideo}{\textit{Supp. Video}\xspace}

\usepackage{pifont}
\usepackage{makecell}
\newlength\savewidth\newcommand\shline{\noalign{\global\savewidth\arrayrulewidth
  \global\arrayrulewidth 1pt}\hline\noalign{\global\arrayrulewidth\savewidth}}
\newcommand{\tablestyle}[2]{\setlength{\tabcolsep}{#1}\renewcommand{\arraystretch}{#2}\centering\small}
